# Supplementary material for: A Proactive Longitudinal Clinical Agent for ICU Monitoring
Source: arXiv:2611.37906 source file (2026-11-27)
Supplement: Supplementary file 1 [file supplementary.tex]

\documentclass[10pt, letter, onecolumn]{arxiv}

\usepackage{kantlipsum, lipsum}
\usepackage{dm-colors}
\usepackage{amsmath}
\usepackage{pstricks, pst-node}
\usepackage{verbatim}
\usepackage{multirow}
\usepackage{array}
\usepackage{longtable}
\usepackage{pdflscape}
\usepackage{scalerel}
\usepackage{booktabs}
\usepackage{enumitem}
\usepackage{xspace}
\usepackage{bm}
\usepackage{bbm}
\usepackage{mathtools}
\usepackage{soul}
\usepackage{epsfig}
\usepackage{graphicx}
\usepackage{amssymb}
\usepackage{colortbl}
\usepackage{csquotes}
\usepackage{setspace}
\usepackage{colortbl}
\usepackage{bbding}
\usepackage{threeparttable}
\usepackage{tabularx,ragged2e}
\usepackage{placeins}
\usepackage{bbding}
%\definecolor{darkpastelgreen}{rgb}{0.01, 0.75, 0.24}
\definecolor{darkpastelgreen}{rgb}{0.13, 0.55, 0.13}
%\definecolor{darkpastelred}{rgb}{0.76, 0.23, 0.13}
\definecolor{darkpastelred}{rgb}{0.55, 0.13, 0.13}
% \definecolor{mygray}{rgb}{0.85, 0.85, 0.85}
\definecolor{mygray}{rgb}{1, 1, 1}
\usepackage{lmodern}
% \usepackage{lstlisting}
%\usepackage[symbol]{footmisc}
\usepackage[hang,flushmargin]{footmisc}

% \usepackage[bibstyle=nature,citestyle=numeric-comp,%
%             natbib=true,backend=biber,maxbibnames=99,%
%             giveninits=false,sorting=none]{biblatex}
% \usepackage{natbib}
\usepackage{nameref}
\usepackage{varioref}
\usepackage{amssymb}% http://ctan.org/pkg/amssymb
\usepackage{pifont}% http://ctan.org/pkg/pifont
\usepackage{rotating}
\usepackage{graphicx}
\newcommand{\cmark}{\ding{51}}%
\newcommand{\xmark}{\ding{55}}%

\usepackage[pagebackref=false,breaklinks=false,%
            colorlinks=true,bookmarks=true,citecolor=ourdarkblue,%
            urlcolor=ourdarkblue,linkcolor=ourdarkblue]{hyperref}
\usepackage[noabbrev,capitalize]{cleveref}
\usepackage{etoc}
\usepackage{lineno}
\usepackage{algorithm}
\usepackage{makecell} 
\usepackage{algpseudocode}
%\addbibresource{references.bib}
%\renewcommand*{\bibfont}{\linespread{0.8}\footnotesize}
% \usepackage[table]{xcolor} % 确保加载了xcolor包
% \definecolor{mygray}{gray}{0.9} % 在这里定义颜色mygray

\usepackage{amsmath}
\usepackage{thmtools}
\usepackage{tcolorbox}
\usepackage{lmodern}

\declaretheoremstyle[
    spaceabove=6pt, spacebelow=6pt,
    headfont=\bfseries, headpunct={.}, headformat={\NAME\ \NUMBER},
    bodyfont=\normalfont,
    % bodyfont=\normalfont\itshape,
    postheadspace=0.5em
]{promptstyle}

\declaretheorem[name=Prompt, style=promptstyle]{prompt}

\tcolorboxenvironment{prompt}{
    colback=gray!10!,
    colframe=gray!75!,
    fonttitle=\bfseries,
    title=Prompt,
    boxrule=0.5pt,
    sharp corners
}

\graphicspath{{figures/}}
\definecolor{mygray}{rgb}{0.85, 0.85, 0.85}
\newcommand{\weidi}[1]{{\textcolor{magenta}{[weidi: #1]}}}
\newcommand{\chaoyi}[1]{{\textcolor{blue}{[chaoyi: #1]}}}
\newcommand{\pengcheng}[1]{{\textcolor{orange}{[Pengcheng: #1]} }}
\newcommand{\shuyu}[1]{{\textcolor{cyan}{[Shuyu: #1]} }}

\newcommand{\change}[1]{{\textcolor{black}{#1}}}
\newcommand{\changetwo}[1]{{\textcolor{red}{#1}}}


\newcommand{\todo}[1]{\textcolor{blue}{\textbf{TODO:} (#1)}}
\newcommand{\mn}[1]{\textcolor{blue}{{(MN: #1)}}}
\newcommand{\one}[1]{\mathbbm{1}_{[#1]}}
\newcommand{\figref}[1]{Fig.~\ref{#1}}
\newcommand{\tabref}[1]{Tab.~\ref{#1}}
\newcommand{\secref}[1]{Sec.~\ref{#1}}
\newcommand{\AlgRef}[1]{Algorithm~\ref{#1}}
\newcommand{\equref}[1]{Equ.~(\ref{#1})}
\newenvironment{rednote}{\par\color{red}}{\par}

\def\eg{{\em e.g.,}}
\def\ie{{\em i.e.,}}
\def\vs{{\em vs.~}}
\def\etc{{\em etc}\xspace}
\def\etal{{\em et al.}\xspace}


\title{\Large{Quantifying the Reasoning Abilities of LLMs \\ on Clinical Cases (Supplementary Information)}}

% -------------  Authors ----------------------
% \author[$\ast$,1]{Anonymous Author List}

% % -------------  Authors ----------------------
\author[1,2,$\ast$]{Pengcheng Qiu} %#1
\author[1,2,$\ast$]{Chaoyi Wu} %#1
% % TO ADD
\author[1]{Shuyu Liu}
\author[3]{Yanjie Fan}
\author[1,2]{Weike Zhao}
\author[4]{Zhuoxia Chen}
\author[4]{\\ \vspace{0.1cm}Hongfei Gu}
\author[4]{Chuanjin Peng}
\author[1,2]{Ya Zhang}
\author[1,2,$\dag$]{Yanfeng Wang} 
\author[1,2,$\dag$]{Weidi Xie}

\affil[1]{\normalsize Shanghai Jiao Tong University, Shanghai, China \authorcr \vspace{0.1cm}}

\affil[2]{\normalsize Shanghai Artificial Intelligence Laboratory, Shanghai, China  \authorcr \vspace{0.1cm}}

\affil[3]{\normalsize Xin Hua Hospital Affiliated to Shanghai Jiao Tong University School of Medicine, Shanghai, China \authorcr\vspace{0.1cm}}

\affil[4]{\normalsize China Mobile Communications Group Shanghai Co., Ltd., Shanghai, China \authorcr \vspace{0.1cm}}



\affil[$\ast$]{\normalsize Equal contributions\hspace{1cm}}
\affil[$\dag$]{\normalsize Corresponding author\authorcr Yanfeng Wang: wangyanfeng622@sjtu.edu.cn; Weidi Xie: weidi@sjtu.edu.cn}




\begin{document}
%\begin{refsection}
% \linenumbers 



\maketitle
% \clearpage

% ========== Figures
% \input{content_npj/07_Figures}

% \clearpage
\appendix
\input{content_npj/06_Appendix}

%\end{refsection}
\clearpage
%\setlength\bibitemsep{3pt}
%\printbibliography
%\balance
\bibliographystyle{unsrt}
% \bibliography{references} % Entries are in the refs.bib file
\end{document}
